# Supplementary material for: LiftRefine: Progressively Refined View Synthesis from 3D Lifting with Volume-Triplane Representations
Source: arXiv:2412.14464 source file (2024-12-19)
Supplement: Supplementary file 1 [file training_inference.tex]

\section{Implementation Details}
\label{sec:training_inference}
\myheading{Training.} To train the reconstructor, we randomly sample 1 to 3 images as input $\mI_{in}$. The target image $\mI_{target}$ is sampled as follows. 
A straightforward strategy is to set $\mI_{target}$ to a random sample in the training dataset. However, we empirically found that this often leads to overfitting. 
To regularize the reconstructor, we instead opt for a probabilistic approach as follows.
We set $\mI_{target}$ to the first input view in $\mI_{in}$ with probability 0.8, and set $\mI_{target}$ to a random sample in the training dataset otherwise. 
This strategy helps reduce view ambiguity during training, which in turn prevents overfitting. 

To train the diffusion model, we randomly select an image $\mI_k$ and its corresponding camera pose $\Psi_{k}$ from the training dataset such that $\mI_k \neq \mI_{target}$. We use the coarse-scale volume feature created from $\mI_{in}$ to render a coarse feature map 
$\mF_k$. We choose $\mI_k$ instead of the target image here in order to train the diffusion model to gain better refinement ability, i.e., to train the diffusion model to predict target views from condition feature maps with high ambiguity in occluded regions.
Once we sample $\mI_{in}$, $\mI_{target}$, $\mI_k$, we train both the reconstructor and the diffusion model jointly in an end-to-end fashion.

\myheading{Inference.} We use progressive inference (Fig. 3 in our main paper) to combine our 3D reconstructor and our 2D diffusion model. Initially, we interpolate $n$ camera poses between the input and target camera pose. The progressive inference process starts by constructing the volume $\mV_{low}^1$ using the reconstructor and the input images $\mI_{in}$. Subsequently, a feature map $\mF^1$ is rendered for the diffusion model to synthesize a novel view image $\mI^1$. Then, $\mI^1$ is fed to the reconstructor to form $\mV_{low}^{2}$ which then renders a novel view feature map $\mF^{2}$. This iterative process continues until we reach the target cameras. In the final step, all intermediate images $\mI_{1:n}$ and $\mI_{in}$ are utilized to reconstruct a final tri-plane feature and render a refined target view. In our main experiment, we employ 200-steps DDIM sampling \cite{song2022denoising} with classifier free guidance $=2.0$ to sample images from the coarse feature map and 1-step progressive inference to render a novel view.

\myheading{Optimization.} We employ the Adam optimizer \cite{kingma2017adam} with a learning rate of $1 \times 10^{-4}$ for our reconstructor and $1 \times 10^{-5}$ for our diffusion model. The reconstructor utilizes a cosine scheduler, while the diffusion optimizer remains constant. We set the maximum 300k training steps and training until there is no improvement. The batch size is 16 and 8 across 4 A100 GPUs for CO3D and Shapenet SRN-Car respectively. In $\mL_{recons}$, we set $\gamma$ to 0.2 for all experiments.

\myheading{Evaluation.}
For Shapenet SRN-Car, we employ the pretrained models from the baselines for inference whenever available. Otherwise, we utilize their reported results for our quantitative analysis. 

For CO3D dataset, we use the pretrained model from ViewsetDiffusion \cite{szymanowicz23viewset_diffusion} and SparseFusion \cite{zhou2023sparsefusion} to evaluate the results with three different random seeds for each experiment. We compare our deterministic and diffusion setting with ViewsetDiffusion \cite{szymanowicz23viewset_diffusion} since they all generate a 3D representation at the end of the inference process. This results in the novel view being view consistent but of lower quality compared to SparseFusion \cite{zhou2023sparsefusion} and our intermediate setting. By contrast, SparseFusion and our intermediate setting only yield 2D images, which achieve much higher image fidelity but suffer from view inconsistency.

We compute the CLIP scores as follows. For text embedding, we use the prompt "A photo of $category$, black background" (e.g., "A photo of hydrant, black background") and ViT-L/14 \cite{radford2021learning} for image embedding extraction. Finally, we calculate the average pairwise cosine similarity between image and text embeddings.
